# Supplementary material for: GPT-Driver: Learning to Drive with GPT
Source: arXiv:2310.01415 source file (2023-12-05)
Supplement: Supplementary file 1 [file x_appendix.tex]

\section{Appendix}
